# Supplementary material for: CataNet: Predicting remaining cataract surgery duration
Source: arXiv:2106.11048 source file (2021-06-21)
Supplement: Supplementary file 1 [file 10_appendix.tex]

\begin{table}[]
    \centering
    \begin{tabular}{lcccc}
    \hline
            & Densenet-full & Resnet-full     & Dense-noet & Resnet-noet \\
                 \hline
    RSD     & $0.99 \pm 0.65$   & $1.04 \pm 0.68$   & $1.28 \pm 0.69$ & $1.19 \pm 0.60$ \\
    RSD-5   & $0.64 \pm 0.56$   & $0.71 \pm 0.47$   & $0.92 \pm 0.58$ & $0.87 \pm 0.40$ \\
    RSD-2   & $0.35 \pm 0.20$   & $0.35 \pm 0.20$   & $0.49 \pm 0.31$ & $0.45 \pm 0.18$ \\
    RSD@Hyd & $1.66 \pm 1.35$   & $1.67 \pm 1.30$   & $1.66 \pm 1.35$ & $1.91 \pm 1.15$ \\
    \hline
    \end{tabular}
    \caption{RSD is the macro mean absolute error RSD throughout the surgery. RSD-2 is average of the last 2 mins. RSD-5 is average of the last 5 mins. RSD@Hyd is average at the end of hydrodissection step. All values are mean $\pm$ standard deviation in minutes.}
    \label{tab:trainingold}
\end{table}

\subsection{Improvement over RSDNet} 

Table~\ref{tab:rsd-exp} shows that CataNet considerably outperforms the baseline methods, even though the underlying models are similar. To better understand the source of the difference in performance, we replace elements that differentiate CataNet from RSDNet one-by-one and show the results in~Table~\ref{tab:training}. In particular, we experiment with (1) CataNet, (2) CataNet using ResNet-152, (3) CataNet's CNN and RNN trained solely to predict RSD, (4) CataNet trained with the same objective as (3) but instead of concatenating the elapsed time to the video frames, we concatenate it to the output of the LSTM layer, (5) RSDNet trained using the Adam optimizer, early-stopping, and sub-epoch evaluation, similarly to CataNet, and (6) RSDNet. First, it can be seen that there is a small difference between (1) and (2), indicating that the usage of DenseNet or ResNet does not play a big role. Further, it can be seen that having the elapsed time at the beginning of the network (3) considerably outperforms having it at the end (4), both in general terms, but particularly after the Hydrodissection step. Finally, RSDNet (6) shows a big improvement from being trained using most of the components from our proposed training strategy (5). We believe that the difference between (4) and (5) can be explained by our RNN being superior to that of the RSDNet and to the fact that we additionally train the RNN and CNN from (4) jointly in an end-to-end manner. In our experiments, this usually improved the results by about 10\%. In conclusion, this experiment shows that CataNet's improvement in performance over RSDNet comes from 1) predicting surgical step and surgeon's experience, 2) having the elapsed time and the very input of the network, and 3) our proposed training strategy. Comparing to TimeLSTM, 2) and 3) are directly applicable, and 1) is applicable to the extent that TimeLSTM only uses step prediction in the training of the CNN.

\begin{table}[t]
    \centering
    \begin{tabular}{lcccccc}
    \hline
          & (1) CataNet & (2) &  (3)  & (4) & (5)  & (6) RSDNet \\
                 \hline
    MAE@Hyd & $\mathbf{1.66 \pm 1.35}$   & $1.67 \pm 1.30$ & $1.99 \pm 1.38$ & $2.28 \pm 1.34$  & $2.09 \pm 1.20$ & $2.32 \pm 1.27$   \\
    MAE-5   & $\mathbf{0.64 \pm 0.56}$   & $0.71 \pm 0.47$ & $0.76 \pm 0.41$ & $0.74 \pm 0.34$ & $1.05 \pm 0.40$ & $1.37 \pm 0.83$ \\
    MAE-2  & $\mathbf{0.35 \pm 0.20}$   & $0.35 \pm 0.20$    & $0.39 \pm 0.28$ & $0.44 \pm 0.20$ & $1.04 \pm 0.34$  & $1.23 \pm 0.53$   \\
    \hline
    \hline
    MAE    & $\mathbf{0.99 \pm 0.65}$   & $1.04 \pm 0.68$  &  $1.11 \pm 0.62$ & $1.34 \pm 0.73$ & $1.44 \pm 0.52$ & $1.59 \pm 0.69$    \\
\hline
    \end{tabular}
    \caption{RSD prediction results for the cataract-101 dataset for our model and the five versions of baseline methods. (2) CataNet using ResNet as CNN. (3) CataNet trained only for RSD. (4) Same as (3) but concatenating the RNN output with the elapsed time. (5) RSDNet trained with our training strategy.}
    \label{tab:training}
\end{table}
